# Supplementary material for: Sparse Gaussian Process Potentials: Application to Lithium Diffusivity in Superionic Conducting Solid Electrolytes
Source: arXiv:2009.13179 ancillary file (2021-05-20)
Supplement: Supplementary file 1 [file sm.pdf]

**Supplemental Material for**  
**“Towards Universal Sparse Gaussian Process Potentials:**  
**Application to Lithium Diffusivity in Superionic Conducting Solid**  
**Electrolytes”**

Amir Hajibabaei, Chang Woo Myung, and Kwang S. Kim\*

(Dated: September 28, 2020)

**DESCRIPTOR AND KERNEL**

The descriptor for the local chemical environment (LCE) of an atom depends only on the relative coordinates of other nearby atoms within a cutoff radius  $r_c$ . For a similarity kernel between two LCEs, the smooth overlap of atomic positions (SOAP) is defined as [1]

$$k(\rho, \rho') = \int d\mathbf{R} \left| \int d\vec{r} \rho(\vec{r}) \rho'(\mathbf{R}\vec{r}) \right|^2 \quad (\text{S1})$$

where  $\mathbf{R}$  is the 3D rotations operator,  $\rho(\vec{r})$  is the atomic density

$$\rho(\vec{r}) = \sum_i \exp(-\alpha |\vec{r} - \vec{r}_i|^2), \quad (\text{S2})$$

and  $\alpha$  is a hyper-parameter. Such a kernel is invariant with respect to all rotations. The above integrals can be carried out analytically, which ignoring a constant multiplier, results in

$$k(\rho, \rho') \propto \sum_{l,m,m'} \frac{1}{2l+1} I_{mm'}^l {}^* I_{mm'}^l \quad (\text{S3})$$

where

$$I_{mm'}^l = \sum_{i,i'} e^{-\alpha(r_i^2 + r_{i'}^2)/2} \iota_l(\alpha r_i r_{i'}) Y_l^m(\hat{n}_i) Y_l^{m'*}(\hat{n}_{i'}), \quad (\text{S4})$$

$r_i = |\vec{r}_i|$ ,  $\hat{n}_i = \vec{r}_i/r_i$ , and  $\iota_l$  is the modified Bessel function of the first kind (Bessel-i). Unfortunately these equations are not computationally efficient because of the dependence of  $I_{mm'}^l$  identities on both environments. In Bartók et al. [1], this is remedied by expansion of the atomic density using an orthonormal radial basis set  $\{g_n\}$

$$\rho(\vec{r}) = \sum_{n,l,m} c_{nlm} g_n(r) Y_l^m(\hat{n}) \quad (\text{S5})$$

---

\* kimks@unist.ac.kr

which transforms the  $I_{mm'}^l$  identities into inner products

$$I_{mm'}^l = \sum_n c_{nlm} c'_{nlm'}{}^* \quad (\text{S6})$$

which in turn transforms the kernel into an inner-product

$$k(\rho, \rho') \propto \sum_{n,n',l} \left( \sum_m \frac{c_{nlm} c'_{nlm'}{}^*}{\sqrt{2l+1}} \right) \left( \sum_{m'} \frac{c'_{nlm'}{}^* c'_{nlm'}}{\sqrt{2l+1}} \right) = \sum_{n,n',l} p_{nn'l} p'_{nn'l}{}^* \quad (\text{S7})$$

Here we achieve the same goal, by considering the series expansion of Bessel-i functions  $\iota_l$  [2],

$$\iota_l(\alpha r_i r_{i'}) = \sum_{n=0}^{\infty} a_{nl} r_i^{2n+l} r_{i'}^{2n+l} \quad (\text{S8})$$

where  $a_{nl} = (\alpha/2)^{2n+l}/(n+l)!n!$ . Using this expansion we get the same expression for  $I_{mm'}^l$  as Eq. S6 with the expansion coefficients already determined:

$$c_{nlm} = \sqrt{a_{nl}} \sum_i e^{-\alpha r_i^2/2} r_i^{2n+l} Y_l^m(\hat{n}_i). \quad (\text{S9})$$

For elimination of discontinuities due to the application of a cutoff we need to modify the descriptor, for instance by the substitution  $e^{-\alpha r_i^2/2} \rightarrow f(r_i; r_c) e^{-\alpha r_i^2/2}$  where  $f$  is a smooth cutoff function with a continuous derivative at  $r_c$ . The simplest choice is  $f(r; r_c) = (1 - r/r_c)^2$ . The  $a_{nl}$  multipliers decrease extremely fast by increasing  $n$  and  $l$ ; therefore it suffices to calculate up to only a few orders of expansion. In our calculations  $\alpha = 1$ ,  $r_c = 8$ , and  $l, n \leq 3$ .

Extension to multi-species environments is straightforward [3]. If the coefficients  $c_{nlm}$  are calculated for each atomic species in the LCE, the total descriptor vector is

$$p_{nn'l}^{\alpha\beta} = \frac{1}{\sqrt{2l+1}} \sum_m c_{nlm}^{\alpha} c_{nlm}^{\beta}{}^* \quad (\text{S10})$$

where  $\alpha$  and  $\beta$  denote the species.

The kernel may be generalized to

$$k(\rho_i, \rho_j) = \mu_{s_i s_j} \left( \sum_{\substack{\alpha, \alpha', \beta, \beta', \\ n, n', l}} [p_{nn'l}^{\alpha\beta}]_i [p_{nn'l}^{\alpha'\beta'}]_j \chi_{\alpha\alpha'} \chi_{\beta\beta'} \right)^{\eta} \quad (\text{S11})$$

where  $\chi_{\alpha\beta}$  is an alchemical similarity kernel between the atomic species in LCEs and  $\mu_{s_i s_j}$  is a kernel which depends on the species of the central atoms  $i, j$  and quantifies the covariance between local energies. Here we have chosen  $\chi_{\alpha\beta} = \delta_{\alpha\beta}$  and  $\mu_{s_i s_j} = \delta_{s_i s_j}$ . The latter corresponds to summation of independent Gaussian processes defined for each atomic species. The exponent  $\eta$  controls the sensitivity of the kernel which is fixed at 4 in our work. Finally, the kernel is normalized by  $k(\rho_i, \rho_j) / \sqrt{k(\rho_i, \rho_i) k(\rho_j, \rho_j)}$ .

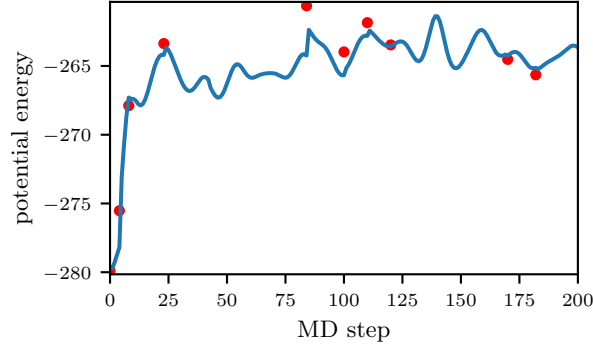

FIG. S1. On-the-fly predicted potential energy of the SGPR model at the beginning of MD. Red bullets indicate the timings and energies of FP calculations.

### TRAINING AND TESTING

For general targets  $\{y_i\}$  and a model's predictions  $\{f_i\}$ , coefficient of determination (CD) of the model is defined by

$$R^2 = 1 - \frac{\sum_i (y_i - f_i)^2}{\sum_i (y_i - \bar{y})^2}. \quad (\text{S12})$$

Since CD is normalized by the variance in the data, it is a more consistent measure than root mean squared error (RMSE). For energies, it is more appropriate to use mean absolute error (MAE) because, unlike forces, energies are not distributed around zero and uniform shift does not affect RMSE.

As the first example in the main text, a SGPR potential is trained on-the-fly with MD, with three different systems:  $\gamma$ -Li<sub>3</sub>PS<sub>4</sub> with  $(1 \times 1 \times 2)$ ,  $\beta$ -Li<sub>3</sub>PS<sub>4</sub> with  $(2 \times 1 \times 1)$ , and Li<sub>7</sub>P<sub>3</sub>S<sub>11</sub> with  $(2 \times 1 \times 1)$  cells. For sampling, the systems were quenched from  $\sim 1500$  K to 700 K in  $\sim 5$  ps by velocity re-scaling and kept at this temperature for  $\sim 45$  ps using a time step of 2 fs. In quenching, there is no time for the crystal to melt (since atoms do not have time to displace too far the crystal becomes only locally disordered) but this local distortion results in stream of diverse LCEs to the sampling algorithm which helps in faster stabilization of the model at the beginning of training. This practice is beneficial but not compulsory. The algorithm FAST (see adaptive sampling algorithms in the main text) is applied in training (see Fig. S1), therefore in total only 456 FP calculations are performed from which only 111 are sampled by the model (as data  $X, Y$ ) and 705 LCEs are sampled as the inducing set ( $z$ ). For the sake of speed, only  $\Gamma$  point is selected for sampling k-space, but afterwards the potential energy and forces are recalculated with a  $2 \times 2 \times 2$

k-point grid only for those 111 data which are included in the model. This corrects the forces by an RMSE of about  $0.04 \text{ eV } \text{\AA}^{-1}$ . In Fig. S2 performance of the model on all 456 examples is demonstrated.

To verify the model with independent data, MLMD simulations at five temperatures in the range 300 to 700 K for 0.8 to 2.2 ns are performed (only for  $\text{Li}_7\text{P}_3\text{S}_{11}$ , same size as training) and  $10^3$  snapshots are randomly selected. Accuracy of the model is tested with these samples in Fig. S3.

In addition, the liquid and glass phase  $\text{Li}_7\text{P}_3\text{S}_{11}$  are simulated with the SGPR model. Testing of the model in these phases is shown in Fig. S4. Since size of the cells in these simulations (672 atoms) are larger than the training systems, the SGPR model slightly underestimates the total energy (by  $\sim 3 \times 10^{-3} \text{ eV}$  per-atom) due to the long-range forces that are excluded because of a finite cutoff radius. Treatment of the long-range forces with ML models is not trivial yet.

To demonstrate that the generated SGPR model is energy-conservative, an MD simulation in NVE ensemble is carried out which is shown in Fig. S5. A nudged elastic band (NEB) calculations is also carried out which is directly compared with DFT in Fig. S6.

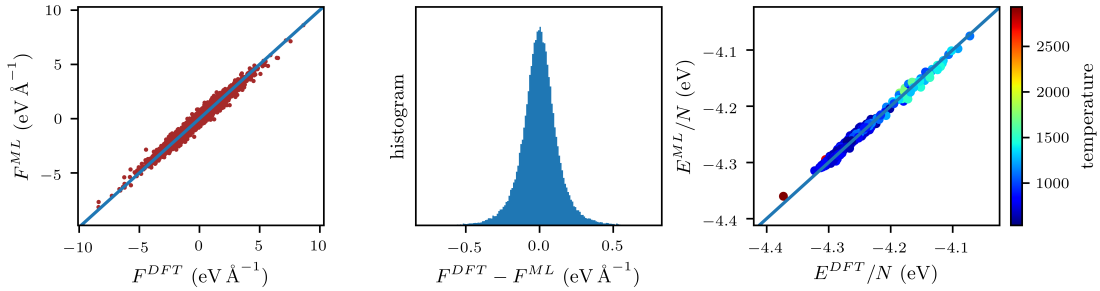

FIG. S2. **Training data:** testing the model trained with  $\text{Li}_3\text{PS}_4$  ( $\alpha$  and  $\beta$ ) and  $\text{Li}_7\text{P}_3\text{S}_{11}$  on all 456 FP calculations which were performed during training. For forces RMSE is  $0.13 \text{ eV } \text{\AA}^{-1}$  and  $R^2 = 0.967$ . For energies MAE is  $3.817 \times 10^{-3} \text{ eV}$  per-atom.

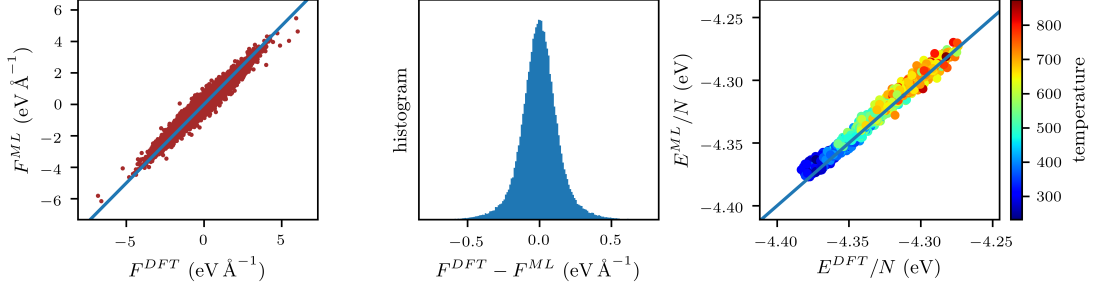

FIG. S3. **Crystal phase:** 1000 samples are randomly selected from extensive MLMD simulations of  $\text{Li}_7\text{P}_3\text{S}_{11}$  at five temperatures in the range 300 to 700 K for 0.8 to 2.2 ns. The number of atoms in these samples is 84. For forces RMSE is  $0.139 \text{ eV } \text{\AA}^{-1}$  and  $R^2 = 0.944$ . For energies MAE is  $3.822 \times 10^{-3} \text{ eV}$  per-atom.

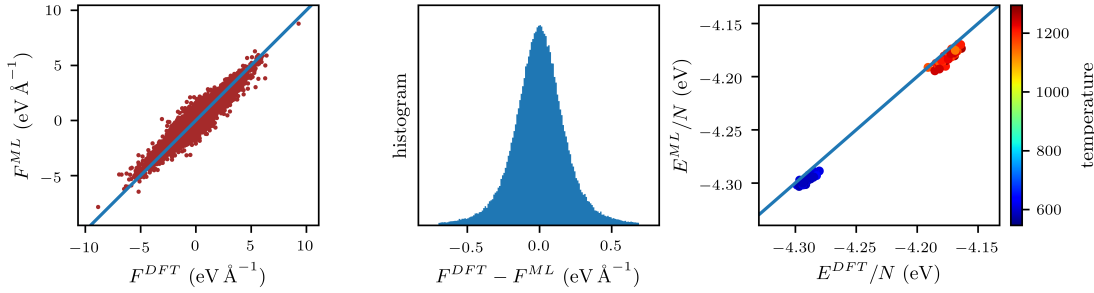

FIG. S4. **Liquid and glass phases:** 50+70 samples are drawn from MLMD simulation of the liquid phase  $\text{Li}_7\text{P}_3\text{S}_{11}$  at 1200 K and glass phase (obtained after melt-quenching) at 600 K for  $\sim 0.2$  ns. The number of atoms in these samples is 672. The errors in these phases are similar. For forces RMSE is  $0.21 \text{ eV } \text{\AA}^{-1}$  and  $R^2 = 0.917$ . For energies MAE is  $6.35 \times 10^{-3} \text{ eV}$  per-atom.

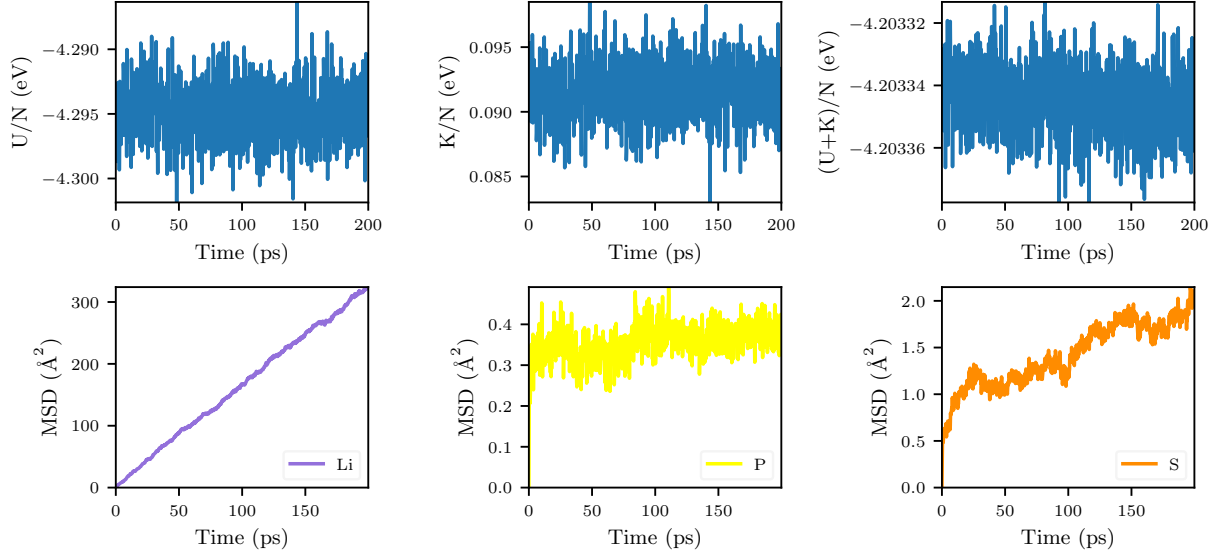

FIG. S5. **Energy conservation:** MLMD simulation of  $\text{Li}_7\text{P}_3\text{S}_{11}$  with 672 atoms in NVE ensemble with velocity-Verlet algorithm. The temperature is  $\sim 700$  K. The per-atoms potential energy, kinetic energy, and total energy are plotted in the first row. The total energy is conserved up to small fluctuations of  $\sim 10^{-5}$  eV per atom which are related to the finite timestep of 2 fs. In the second row, MSDs of atoms from their initial positions are plotted.

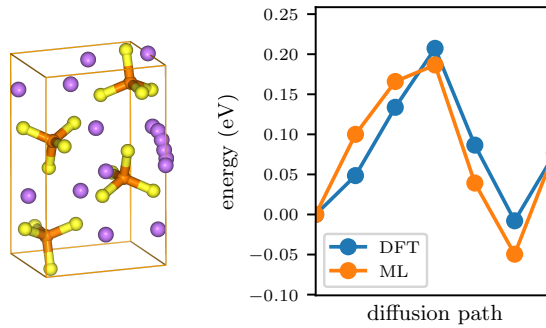

FIG. S6. Nudged elastic band calculations for Li hopping to a neighboring vacancy (created by Li removal) in  $\gamma\text{-Li}_3\text{PS}_4$  with DFT and ML potentials.  $(2 \times 2 \times 2)$  k-point grid is applied in DFT calculations.

# LARGE SCALE MLMD SIMULATIONS

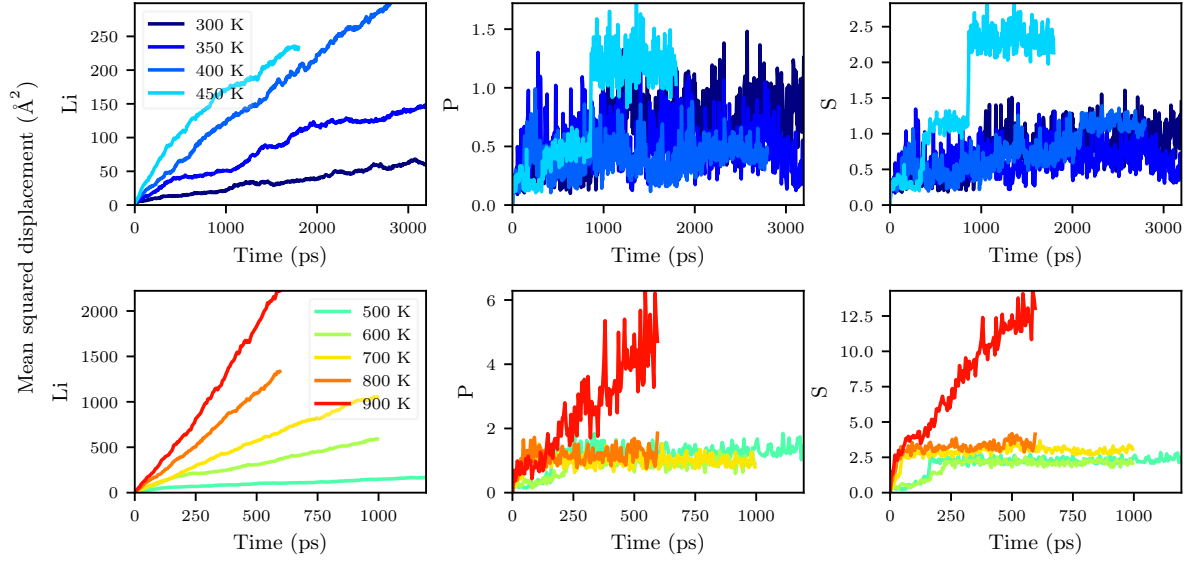

FIG. S7. Mean squared displacements of atoms in  $\text{Li}_7\text{P}_3\text{S}_{11}$  system (with 672 atoms) during the MD simulation in the NPT ensemble with temperatures ranging from 300 to 900 K. The jumps in the MSD of P and S atoms are associated with a crystal-crystal ( $\alpha \rightarrow \beta$ ) phase transition. The crystal melts at 900 K.

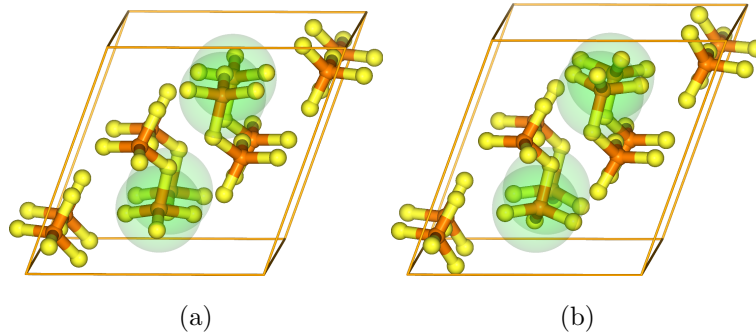

FIG. S8. Relaxed (a)  $\alpha$  and (b)  $\beta$  cells of  $\text{Li}_7\text{P}_3\text{S}_{11}$ , while Li atoms are removed for clarity. The rotated  $\text{PS}_4$  tetrahedra are highlighted with green.

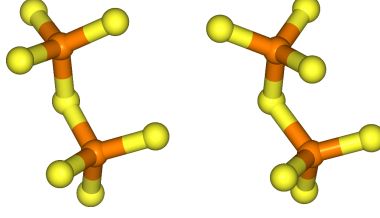

FIG. S9. Preferred orientations of  $P_2S_7$  double-tetrahedra in  $\alpha$  (left) and  $\beta$  (right) phases of  $Li_7P_3S_{11}$ .

## DIFFUSION MECHANISMS

Diffusion pathways are visualized in Fig. S10. In  $\alpha$  phase, the diffusion of Li atoms is highly concerted and chain-like. By reorientation of some of  $PS_4$  tetrahedra in  $\beta$  phase, this chain-like diffusion is somewhat scattered. For a more quantitative explanation, the directional MSD along  $\hat{n}$  is defined by

$$MSD_{\hat{n}}(t) = \frac{1}{N} \sum_{i=1}^N |\Delta \vec{r}_i(t) \cdot \hat{n}|^2. \quad (S13)$$

As shown in Fig. S10c, the diffusivity is the largest along the  $\vec{a}$ -axis in both phases. The main difference is that the diffusivity along  $\vec{b}$  and  $\vec{c}$  axes are almost equal in  $\alpha$  phase, while in  $\beta$  phase this symmetry is clearly broken.

## COMPUTATIONAL PERFORMANCE

For a system with  $N$  atoms, the computational cost of predicting energy and forces with the SGPR model is  $\mathcal{O}(N)$ , while the complexity of FP calculations is  $\mathcal{O}(N^3)$  or at best  $\mathcal{O}(N^2 \log N)$ . The elapsed time for FP calculations of the energy and forces for a system with 672 atoms was 9718s using VASP with 80 cores, while the elapsed time for the same calculation with SGPR was 5.3s using only 20 cores. The cost defined by elapsed  $\times$  cores/ $N$  is  $\sim 0.15$ s for SGPR which is better than FP calculations by a factor of  $\mathcal{O}(10^4)$ .

## GRAIN BOUNDARIES AND LONG-RANGE DIFFUSIVITY

Consider an infinite 1D lattice where  $p_j = \exp(-\varepsilon_j/k_B T)$  is the probability that a random walker will jump over the edge connecting  $j$  and  $j+1$  vertices ( $p_j = p_{j \rightarrow j+1} = p_{j+1 \rightarrow j}$ ) and  $\varepsilon_j$  is the energy barrier. If  $p_j = p$  for all  $j$ , then  $D = \nu a^2 p$  is the diffusion coefficient for random walkers where  $a$  is the lattice spacing and  $\nu$  is the frequency of the jump trials. In general case where  $p_j$  is



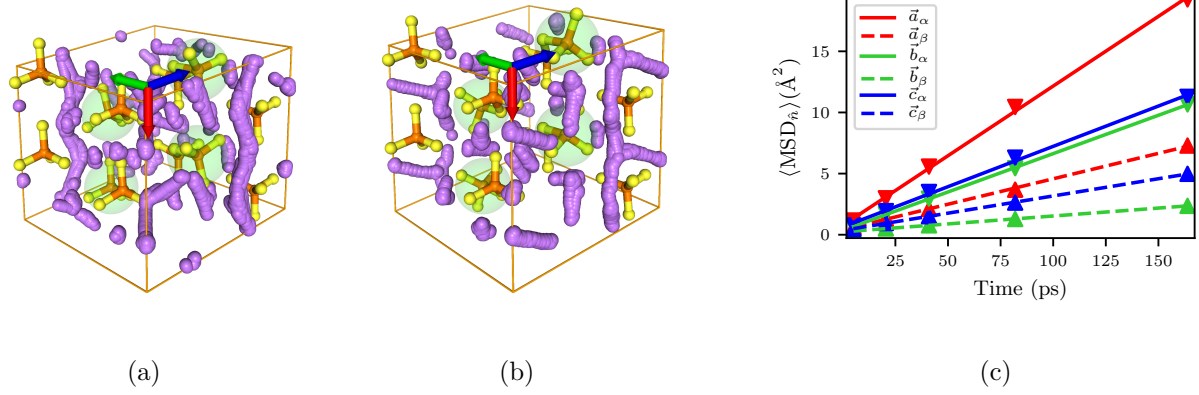

FIG. S10. Time-lapse of the Li positions over a few hundred ps in (a)  $\alpha$  and (b)  $\beta$  phases of  $\text{Li}_7\text{P}_3\text{S}_{11}$  with a  $2 \times 1 \times 1$  cell at 300 K. (c) Directional MSD in  $\alpha$  and  $\beta$  phases sampled by MD with a  $4 \times 2 \times 2$  cell at 450 K. The respective unit cell vectors ( $\vec{a}, \vec{b}, \vec{c}$ ) are indicated with red, green and blue vectors in (a) and (b).

non-uniform, the diffusion coefficient becomes  $D = \nu a^2 p^f$  and  $\varepsilon^f = -k_B T \log(p^f)$  is the effective energy barrier which can be calculated (analogous to series of resistors) from following

$$\frac{1}{p^f} = \left\langle \frac{1}{p_j} \right\rangle = \left\langle \exp(\varepsilon_j / k_B T) \right\rangle. \quad (\text{S14})$$

As a simple model for a crystal with grain boundaries, assume that one out of every  $l$  edge has a different energy barrier  $\varepsilon_g$ ; otherwise the energy barrier is equal to  $\varepsilon_a$ . The effective energy barrier becomes

$$\varepsilon^f = -k_B T \log \left( \frac{l}{(l-1) \exp(\varepsilon_a / k_B T) + \exp(\varepsilon_g / k_B T)} \right). \quad (\text{S15})$$

If  $\frac{\varepsilon_a}{k_B T}, \frac{\varepsilon_g}{k_B T}, \frac{1}{l} \ll 1$ , then

$$\varepsilon^f \approx \varepsilon_a + \frac{\varepsilon_g - \varepsilon_a}{l} \quad (\text{S16})$$

which readily shows how the activation energy for long-range diffusion is related to the spacing of the grain boundaries.

TABLE S1. **Ternary solid electrolytes:** 22 promising ternary solid electrolytes obtained after filtering of about 300 candidates. Diffusivities are obtained with MLMD in NPT ensemble for  $\sim 100$  ps. Modeling and MLMD for  $\text{Li}_7\text{P}_3\text{S}_{11}$  is repeated here which resulted in a slightly lower conductivity ( $\sim 20$ ) than previous simulation ( $\sim 35$  in main text) because it is obtained by extrapolation while in the main text it is obtained by direct simulation at 300 K. The first column is the ID of crystal in the **materialsproject** [4] repository.

| mp-ID      | formula                                    | ML error<br>(eV $\text{\AA}^{-1}$ ) | $D$ ( $\text{\AA}^2/\text{ps}$ ) at given temperature (K) |       |       |       |       |       |      |      | $E_a$<br>(eV) | $\sigma$ (mS $\text{cm}^{-1}$ )<br>at 300 K |
|------------|--------------------------------------------|-------------------------------------|-----------------------------------------------------------|-------|-------|-------|-------|-------|------|------|---------------|---------------------------------------------|
|            |                                            |                                     | 400                                                       | 500   | 600   | 700   | 800   | 900   | 1000 | 1200 |               |                                             |
| mp-1211324 | $\text{Li}_7\text{PS}_6$                   | 0.12                                |                                                           |       | 0.15  |       | 0.29  |       | 0.54 | 0.83 | 0.18          | 65.2                                        |
| mp-1097036 | $\text{Li}_3\text{PS}_4$                   | 0.14                                |                                                           | 0.068 | 0.14  | 0.28  | 0.46  |       |      |      | 0.23          | 20.2                                        |
| mp-641703  | $\text{Li}_7\text{P}_3\text{S}_{11}$       | 0.18                                |                                                           |       | 0.12  | 0.2   | 0.32  |       | 0.61 |      | 0.21          | 20.1                                        |
| mp-768197  | $\text{Li}_5\text{SbS}_4$                  | 0.16                                |                                                           |       | 0.1   | 0.18  | 0.31  |       |      |      | 0.23          | 18.4                                        |
| mp-1147621 | $\text{Li}_3\text{InBr}_6$                 | 0.15                                | 0.018                                                     | 0.057 | 0.13  |       |       |       |      |      | 0.2           | 16.1                                        |
| mp-28327   | $\text{LiGaBr}_3$                          | 0.2                                 |                                                           | 0.049 | 0.11  |       |       |       |      |      | 0.21          | 7.6                                         |
| mp-756427  | $\text{Li}_5\text{SbS}_4$                  | 0.17                                |                                                           |       |       | 0.086 | 0.19  | 0.26  | 0.37 |      | 0.26          | 6.0                                         |
| mp-685863  | $\text{Li}_4\text{SiO}_4$                  | 0.18                                |                                                           |       |       |       | 0.093 | 0.2   | 0.32 | 0.53 | 0.3           | 3.1                                         |
| mp-1195718 | $\text{Li}_4\text{SnS}_4$                  | 0.12                                |                                                           |       |       |       | 0.18  | 0.32  | 0.37 | 0.74 | 0.29          | 2.3                                         |
| mp-766409  | $\text{Li}_3\text{BiS}_3$                  | 0.15                                |                                                           |       | 0.034 | 0.077 | 0.12  |       | 0.29 |      | 0.27          | 2.1                                         |
| mp-29009   | $\text{Li}_2\text{MgBr}_4$                 | 0.13                                |                                                           |       | 0.045 | 0.096 | 0.18  |       |      |      | 0.28          | 1.4                                         |
| mp-38684   | $\text{Li}_2\text{MgCl}_4$                 | 0.12                                |                                                           |       | 0.047 | 0.095 | 0.21  |       | 0.46 |      | 0.3           | 1.3                                         |
| mp-760415  | $\text{Li}_3\text{SbS}_4$                  | 0.14                                |                                                           |       |       |       | 0.2   |       | 0.57 | 0.98 | 0.33          | 0.83                                        |
| mp-1194700 | $\text{Li}_4\text{SnSe}_4$                 | 0.13                                |                                                           |       |       |       | 0.15  | 0.3   | 0.41 | 0.8  | 0.33          | 0.6                                         |
| mp-1222582 | $\text{Li}_4\text{GeS}_4$                  | 0.13                                |                                                           |       |       |       | 0.14  | 0.31  | 0.4  | 0.93 | 0.38          | 0.24                                        |
| mp-1001069 | $\text{Li}_{48}\text{P}_{16}\text{S}_{61}$ | 0.17                                |                                                           |       | 0.027 | 0.083 | 0.17  |       |      |      | 0.38          | 0.22                                        |
| mp-1177520 | $\text{Li}_3\text{SbS}_3$                  | 0.18                                |                                                           |       | 0.018 | 0.058 | 0.18  |       | 0.39 |      | 0.38          | 0.2                                         |
| mp-775806  | $\text{Li}_3\text{SbS}_3$                  | 0.16                                |                                                           |       |       |       | 0.084 | 0.16  | 0.27 | 0.49 | 0.36          | 0.19                                        |
| mp-38487   | $\text{Li}_7\text{BiO}_6$                  | 0.092                               |                                                           |       |       |       | 0.041 | 0.079 | 0.12 | 0.25 | 0.37          | 0.17                                        |
| mp-753720  | $\text{Li}_3\text{BiS}_3$                  | 0.15                                |                                                           |       |       |       | 0.08  | 0.14  | 0.21 | 0.51 | 0.39          | 0.079                                       |
| mp-29008   | $\text{Li}_6\text{MgBr}_8$                 | 0.097                               |                                                           |       | 0.019 | 0.052 | 0.13  | 0.23  |      |      | 0.41          | 0.077                                       |
| mp-757150  | $\text{Li}_5\text{BiS}_4$                  | 0.17                                |                                                           |       | 0.02  | 0.12  | 0.2   | 0.41  |      |      | 0.46          | 0.049                                       |

- 
- [1] A. P. Bartók, R. Kondor, and G. Csányi, On representing chemical environments, *Physical Review B* **87**, 184115 (2013).
- [2] G. N. G. N. Watson, *A treatise on the theory of Bessel functions* (Cambridge University Press, 1995) p. 804.
- [3] S. De, A. P. Bartók, G. Csányi, and M. Ceriotti, Comparing molecules and solids across structural and alchemical space, *Physical Chemistry Chemical Physics* **18**, 13754 (2016).
- [4] A. Jain, S. P. Ong, G. Hautier, W. Chen, W. D. Richards, S. Dacek, S. Cholia, D. Gunter, D. Skinner, G. Ceder, and K. A. Persson, Commentary: The materials project: A materials genome approach to accelerating materials innovation (2013).
